# Supplementary material for: HICO-DET-SG and V-COCO-SG: New Data Splits for Evaluating the Systematic Generalization Performance of Human-Object Interaction Detection Models
Source: arXiv:2305.09948 source file (2024-04-12)
Supplement: Supplementary file 1 [file 8_4_appendix_old.tex]

%%%% Copied on March 30, 2023

\section{Further results and discussions}
% \label{discussions}

% \subsection{Difference between HICO-DET-SG and V-COCO-SG}
% Comparing two datasets, there are larger gaps between the original and the systematic generalization splits of V-COCO compared to HICO-DET.
% We speculate that the cause of this gap is the difference in the number of images and HOIs in the dataset. As shown in Table \ref{table_sg_stat}, HICO-DET-SG train data contains about 5.6 times as many images and about 12.6 times as many HOIs as the train data of V-COCO-SG. This means that there are more examples for one object-interaction combination in HICO-DET-SG train data, although the data has only 3.4 times as many variety of object-interaction combination classes. Therefore the models tend to achieve higher systematic generalization on HICO-DET-SG compared to V-COCO-SG.

% \subsection{Comparison across models}
% Each model showed different performance on systematic generalization splits.
% HOTR could not generalize at all as they achieved almost 0\% mAP when its encoder and decoder are not pre-trained with object detection task, and achieved less than 3\% mAP even with its encoder and decoder pre-trained. 
% QAHOI also achieved low mAPs around 5\% to show its inability to systematic generalization. 
% However, QPIC generalizes to novel combinations to some extent especially when using pre-trained DETR weights: they achieved around 20\% mAPs on HICO-DET-SG splits. 
% % It also performed better than the others without pre-training, achieving over 10\% mAPs.
% STIP showed the best SG performance among all the models on both HICO-DET-SG and V-COCO-SG with pre-training. This may be because STIP has two-stage architecture. Instance and interaction detector is less affected by each other as they are independent. In other computer vision tasks, this type of modularity is proved to improve systematic generalization ability~\citep{Yamada_2022}.

% \subsection{Importance of pre-trained encoder and decoder}
% For three models except QAHOI, pre-training its encoder and decoder with the weights of DETR trained on object detection task plays a key role in improving systematic generalization performance.
% The accuracies on HICO-DET changed from around 0.4\% to around 2.7\% for HOTR, from around 12.1\% to around 20.8\% for QPIC and from 0.0\% to around 23.2\% for STIP.
% Also the accuracies on V-COCO changed from around 0.2\% to around 2.1\% for HOTR, from around 0.6\% to around 3.8\% for QPIC and from around 0.0\% to 6.3\% for STIP.

% Generally vision Transformers require a lot of training to achieve high performance when trained from scratch~\citep{Khan_2021}. So it is natural that without pre-training, the Transformer-based HOI detectors cannot solve merely HOI detection task nor systematic generalization.
% Especially STIP performed quite badly without pre-training because the number of training epochs is much smaller (30 epochs) than the others (100 epochs).
% For the three models, pre-trained initial weights of encoder and decoder contributes to improving systematic generalization accuracy as well as HOI detection task itself. 
% % Especially QPIC on HICO-DET-SG almost doubled the systematic generalization mAP with pre-training, from around 12.1\% to around 20.8\%.
% In this paper we could not evaluate pre-trained QAHOI because the network is designed only for HOI detection task and it is hard to obtain pre-trained weights from other tasks such as object detection. If we modify the final part of QAHOI so that it can be trained with other tasks, we may be able to get better systematic generalization score with the pre-trained weights.

\subsection{Evaluation on the train data}
In order to make sure that the models are well-trained, we evaluated accuracies on the train data. 
In Table~\ref{table_HICO-DET_train} and Table~\ref{table_VCOCO_train}, we show mAP accuracies on the train data as well as the test data for HICO-DET-SG and V-COCO-SG, respectively (the right half of the tables are equivalent to 
% Figure \ref{fig_HICO-DET} and Figure \ref{fig_VCOCO}). 
Figure \ref{fig_combined}.
For both datasets and for all the models, mAPs on the train data of SG splits are coequal to or slightly better than the original splits.
This is probably because the train data of SG splits contain less variety of triplets: in HICO-DET-SG there are only 540 combinations of objects and interactions out of 600 combination contained in the original dataset, and in V-COCO-SG there are only 160 out of 228.

% \subsection{Qualitative analysis}
% In order to further reveal the difficulty of systematic generalization in HOI detection, we analyze the failure cases here. Figure \ref{failure_cases} (a), (b) and (c) show the outputs of pre-trained STIP trained and tested on HICO-DET-SG split3, which has the highest mAP among all models and all SG splits.

% Figure \ref{failure_cases} (a) shows an example of predicting wrong interaction class, which is the most frequently observed type of errors. In this example the model predicts the interaction as \textbf{straddle}, even though the correct class is \textbf{wash}. 
% The \textless human, \textbf{straddle}, \underline{horse}\textgreater \hspace{0mm} triplet appears in the train data but the \textless human, \textbf{wash}, \underline{horse}\textgreater \hspace{0mm} triplet appears only in the test data (\textbf{wash} interaction appears with other objects in the train data).
% The model predicts the interaction depending just on the object class (\underline{horse}), i.e., the model cannot generalize to the novel combination \textless human, \textbf{wash}, \underline{horse}\textgreater \hspace{0mm}.

% Figure \ref{failure_cases} (b) shows an example of detecting wrong object. The model predicts an irrelevant region as a wrong class, \underline{bench}, even though it should detect a \underline{bed} under the person in the image. 
% The \textless human, \textbf{lie on}, \underline{bench}\textgreater \hspace{0mm} triplet appears in the train data but the \textless human, \textbf{lie on}, \underline{bed}\textgreater \hspace{0mm} triplet appears only in the test data (\underline{bed} appears with other interactions in the train data).
% This result shows not only that the model cannot generalize to the novel combination but also that the interaction decoder predicts the \textbf{lie on} interaction depending mainly on the visual cue of the human posture, not on the visual cue of the object nor on the positional relationships.

% Figure \ref{failure_cases} (c) shows an example of wrong class prediction for both objects and interaction. The model predicts the \underline{tennis racket} as a \underline{baseball bat} and predicts \textbf{swing} as \textbf{hit}. 
% The \textless human, \textbf{hit}, \underline{baseball bat}\textgreater \hspace{0mm} triplet appears in the train data but the \textless human, \textbf{swing}, \underline{tennis racket}\textgreater \hspace{0mm} triplet appears only in the test data (moreover, \textless human, \textbf{swing}, \underline{baseball bat}\textgreater \hspace{0mm} triplet appears in the train data but \textless human, \textbf{hit}, \underline{tennis racket}\textgreater \hspace{0mm} triplet does not appear in the train data).
% The model detects the object as a \underline{baseball bat} at the first stage, and then at the second stage it predicts the interaction as \textbf{hit} based on the detection results because \underline{baseball bat} frequently appeared with the \textbf{hit} interaction in the train data.

% \begin{figure*}[htbp]
% \begin{minipage}[b]{0.32\columnwidth}
%   \centering
%    \includegraphics[width=0.8\columnwidth]{images/interaction_error.pdf}
%    % \caption{An example of predicting wrong interaction class. The model predicts the interaction as \textbf{straddle}, even though the correct class is \textbf{wash}.}
%     \label{interaction_error}
% \end{minipage}
% \hspace{-0.01\columnwidth}
% \begin{minipage}[b]{0.335\columnwidth}
%   \centering
%    \includegraphics[width=\columnwidth]{images/object_error.pdf}
%     \vspace{-11pt}
%    % \caption{An example of detecting wrong object. The model predicts an irrelevant region as a wrong class, \underline{bench}, even though it should detect a \underline{bed} under the person in the image.}
%     \label{object_error}
% \end{minipage}
% \hspace{0.01\columnwidth}
% \begin{minipage}[b]{0.31\columnwidth}
%   \centering
%    \includegraphics[width=\columnwidth]{images/both_error.pdf}
%     \vspace{-12pt}
%    % \caption{An example of wrong class prediction for both objects and interaction. The model predicts \textless human, \textbf{hit}, \underline{baseball bat}\textgreater \hspace{0mm} triplet even though the correct answer is \textless human, \textbf{swing}, \underline{tennis racket}\textgreater \hspace{0mm} triplet.}
%     \label{both_error}
% \end{minipage}
% \caption{Three failure cases of pre-trained STIP trained and tested on HICO-DET-SG split3. (a) An example of predicting wrong interaction class. The model predicts the interaction as \textbf{straddle}, even though the correct class is \textbf{wash}. (b) An example of detecting wrong object. The model predicts an irrelevant region as a wrong class, \underline{bench}, even though it should detect a \underline{bed} under the person. (c) An example of wrong class prediction for both objects and interaction. The model predicts \textless human, \textbf{hit}, \underline{baseball bat}\textgreater \hspace{0mm} triplet even though the correct answer is \textless human, \textbf{swing}, \underline{tennis racket}\textgreater \hspace{0mm} triplet.}
% \label{failure_cases}
% \end{figure*}

% Figure \ref{qahoi_hico} shows two examples of QAHOI outputs on HICO-DET-SG. In (a), the ground truth answer is \textless person, \textbf{sit at}, \underline{bed}\textgreater \hspace{0mm} triplet but the model misclassifies the interaction as \textbf{lie on}, probably because the interaction frequently appears with \underline{bed} in the train data. In (b), the model outputs \textbf{hit} interactions which often exists between human and \underline{baseball bat}, even though we want the model to classify it as \textbf{carry}. In addition, the model simply misclassifies the object as \underline{frisbee} instead of \underline{baseball bat}. This may be because the model detects objects depending on interactions around it rather than the visual cue of the object itself. In train data,
% \underline{frisbee} frequently appears with \textbf{carry} or \textbf{hold} interactions.
% To summarize, QAHOI tend to detect interactions depending on co-occurring object classes rather than the visual cue of the interaction itself. This makes it difficult for the model to generalize to unseen combinations.
% We assume there are two reason for this poor performance.
% First one is the lack of pre-training, as mentioned above. It is hard for the Transformer-based model to learn from limited number of images and HOI examples without pre-trained weights.
% Second reason is that the QAHOI model limits the source of feature extraction for computational efficiency. It only gathers features from anchor points in the image which represent high objectness scores. This may lead to classifying interactions depending on features regarding co-occurring objects, rather than on features regarding the interaction itself.

\begin{landscape}
\begin{table}
\caption{Comparison of systematic generalization performances on HICO-DET-SG data splits. We show mAPs (\%) for both train and test data, which are higher the better (the right half of this table is equivalent to Figure \ref{fig_combined} (a)). The values reported in the original papers are written in brackets. The term ``pre-train'' means that the initial weights of the model's encoder and decoder are copied from DETR~\citep{carion_2020} trained on object detection. Test accuracies significantly decreased on HICO-DET-SG compared to original HICO-DET.}
\label{table_HICO-DET_train}
\centering
\begin{tabular}{c|cccccccc|cccccccc}
 \toprule
  & \multicolumn{8}{c|}{Evaluation on train data (reference)} & \multicolumn{8}{c}{\textbf{Evaluation on test data (main)} } \\
 % \cmidrule{2-11}
 & \multicolumn{2}{c}{HOTR} & \multicolumn{2}{c}{QPIC} & QAHOI & FGAHOI & \multicolumn{2}{c|}{STIP} & \multicolumn{2}{c}{HOTR} & \multicolumn{2}{c}{QPIC} & QAHOI & FGAHOI & \multicolumn{2}{c}{STIP} \\
pre-train & \xmark & \checkmark & \xmark & \checkmark & \xmark & \xmark & \xmark & \checkmark & \xmark & \checkmark & \xmark & \checkmark & \xmark & \xmark & \xmark & \checkmark \\
\midrule
HICO-DET & 30.54 & 44.80 & 33.29 & 46.28 & 50.23 & 55.82 & 13.47 & 32.23 & 17.63 & 26.30 & 21.70 & 29.59 & 35.30 & 36.91 & 13.21 & 31.57\\
(reported) & & & & & & & & & &(25.73)& &(29.90)&(35.78) & (37.18) & & (32.22) \\
\midrule
SG split1 & 33.92 & 46.03 & 34.05 & 49.70 & 52.94 & 58.97 & 13.69 & 33.17 & 0.33 & 2.81 & 11.23 & 21.94 & 5.78 & 6.14 & 0.00 & 24.53 \\
% \hline %\midrule
SG split2 & 31.48 & 42.04 & 30.23 & 48.28 & 51.50 & 55.95 & 15.13 & 34.44 & 0.40 & 2.97 & 12.87 & 19.98 & 5.23 & 5.93 & 0.00 & 24.14 \\
SG split3 & 32.05 & 44.91 & 35.54 & 47.90 & 48.27 & 54.72 & 13.25 & 30.61 & 0.62 & 3.01 & 15.43 & 20.58 & 5.98 & 6.83 & 0.00 & 26.19  \\
% \hline
Average & 32.48 & 44.33 & 33.30 & 48.63 & 50.90 & 56.55 & 14.02 & 32.74 & 0.45 & 2.93 & 13.18 & 20.83 & 5.66 & 6.30 & 0.00 & 24.95 \\
\bottomrule
\end{tabular}
\end{table}
% \end{landscape}



% \begin{landscape}
\begin{table}
\caption{Comparison of systematic generalization performances on V-COCO-SG data splits. We show mAPs (\%) for both train and test data, which are higher the better (the right half of this table is equivalent to Figure \ref{fig_combined} (b)). The values reported in the original papers are written in brackets. ``pre-train'' means that the initial weights of the model's encoder and decoder are copied from DETR~\citep{carion_2020} trained on object detection. Test accuracy significantly decreased on V-COCO-SG data splits compared to original V-COCO for all the models.}
\label{table_VCOCO_train}
\centering
\begin{tabular}{c|cccccccc|cccccccc}
 \toprule
  & \multicolumn{8}{c|}{Evaluation on train data (reference)} & \multicolumn{8}{c}{\textbf{Evaluation on test data (main)} } \\
 % \cmidrule{2-11}
 & \multicolumn{2}{c}{HOTR} & \multicolumn{2}{c}{QPIC} & QAHOI & FGAHOI & \multicolumn{2}{c|}{STIP} & \multicolumn{2}{c}{HOTR} & \multicolumn{2}{c}{QPIC} & QAHOI & FGAHOI & \multicolumn{2}{c}{STIP} \\
pre-train & \xmark & \checkmark & \xmark & \checkmark & \xmark & \xmark & \xmark & \checkmark & \xmark & \checkmark & \xmark & \checkmark & \xmark & \xmark & \xmark & \checkmark \\
\midrule
Original V-COCO & 28.23 & 64.72 & 30.61 & 65.63 & 43.81 & 52.19 & 19.10 & 72.89 & 24.26 & 62.54 & 27.64 & 63.41 & 40.74 & 45.23 & 18.43 & 70.43 \\
(mAP in the original paper) & & & & & & & & & &(63.8)& &(61.0)&  & (61.2) & & (70.7)\\
\midrule
V-COCO-SG split1 & 30.57 & 65.79 & 31.24 & 67.25 & 45.52 & 54.04 & 23.51 & 71.91 & 0.31 & 2.23 & 1.12 & 4.22 & 2.69 & 3.32 & 0.17 & 6.87 \\
V-COCO-SG split2 & 31.53 & 67.28 & 32.53 & 68.43 & 43.96 & 54.00 & 20.04 & 74.38 & 0.29 & 3.02 & 0.68 & 4.85 & 1.92 & 2.97 & 0.00 & 6.27 \\
V-COCO-SG split3 & 28.21 & 61.07 & 29.83 & 60.47 & 42.88 & 53.32 & 22.41 & 73.43 & 0.38 & 2.13 & 0.39 & 2.96 & 1.84 & 3.13 & 0.00 & 6.91\\
Average over SG splits & 30.10 & 64.71 & 31.20 & 65.38 & 44.12 & 53.79 & 21.99 & 73.24 & 0.33 & 2.46 & 0.73 & 4.08 & 2.15 & 3.14 & 0.06 & 6.68 \\
\bottomrule
\end{tabular}
\end{table}
\end{landscape}



% \subsection{limitation}
